# Supplementary material for: Bridging classical and quantum approaches in optical polarimetry: Predicting polarization-entangled photon behavior in scattering environments
Source: arXiv:2411.06134 ancillary file (2024-11-09)
Supplement: Supplementary file 1 [file supplementary_material.pdf]

# Supplementary material:
# Bridging classical and quantum approaches in optical polarimetry: Predicting polarization-entangled photon behavior in scattering environments

**Vira R. Besaga[a,*], Ivan V. Lopushenko[b,*], Oleksii Sieryi[b], Alexander Bykov[b], Frank Setzpfandt[a,c], Igor Meglinski[d]**

[a]Friedrich Schiller University Jena, Institute of Applied Physics & Abbe Center of Photonics, Albert-Einstein-Str. 6, Jena, 07745, Germany

[b]University of Oulu, Opto-Electronics and Measurement Techniques, P.O. Box 4500, Oulu, FI-90014, Finland

[c]Fraunhofer Institute for Applied Optics and Precision Engineering IOF, Albert-Einstein-Str. 7, Jena, 07745, Germany

[d]Aston University, College of Engineering and Physical Sciences, Birmingham, B4 7ET, UK

*Correspondence to vira.besaga@uni-jena.de and ivan.lopushenko@oulu.fi. These two authors contributed equally to this work.

## S1 Implemented Monte Carlo model

### *S1.1 Concept and physical background*

Within a turbid scattering medium, each photon can follow a plethora of different trajectories defined by the material properties. In biophotonic and atmospheric radiative transfer-based Monte Carlo (MC) models, these properties are: scattering coefficient $\mu_s$, scattering anisotropy factor $g$, absorption coefficient $\mu_a$ and mean refractive index $n$.[1] These parameters ultimately depend on the material's internal structure via concepts of the scattering phase function, corresponding cross-sections and their averaged values obtained by means of statistical electromagnetics.[2] In particular, the higher the scattering coefficient $\mu_s$ and the lower the forward scattering anisotropy factor $g$ are, the broader angular range of the photon scattering directions is.

In order to reliably model the interaction of light with such a medium, we define the indicated material's optical properties, define characteristics of both light source and detector, and sample a statistically significant amount of possible trajectories ($N_{ph} > 10^5$) that photons can follow during propagation.[3] It means that generation of photon packets, their propagation through the sample under study, and detection are consequentially simulated. Each $j$-th photon packet ($j = [1...N_{ph}]$) is characterized by a statistical weight $W_j$, position in Cartesian coordinates $\mathbf{r}_j = (x_j, y_j, z_j)$, propagation direction $\mathbf{s}_j$, and the polarization state. Here, the Cartesian coordinate system $(x, y, z)$ is associated with the scattering medium: $z$ axis is orthogonal to the medium boundaries which are assumed to be plane-parallel. Statistical weight is proportional to the intensity of the photon packet and initially follows the intensity distribution of the modelled light source, which is unit for a plane wave. In the course of the photon packet propagation, its weight is attenuated with respect to Beer-Lambert law.[4] Explicit definition of the propagation direction of the photon packet at source aims at modeling complex optical beams, which e.g. carry optical angular momentum.[5]

Optical properties of the sample medium define the probabilities of individual photon packets to change their direction due to scattering events or to be lost (to have its statistical weight reduced) due to absorption. The detection in this work assumes collection of all photon packets with a single

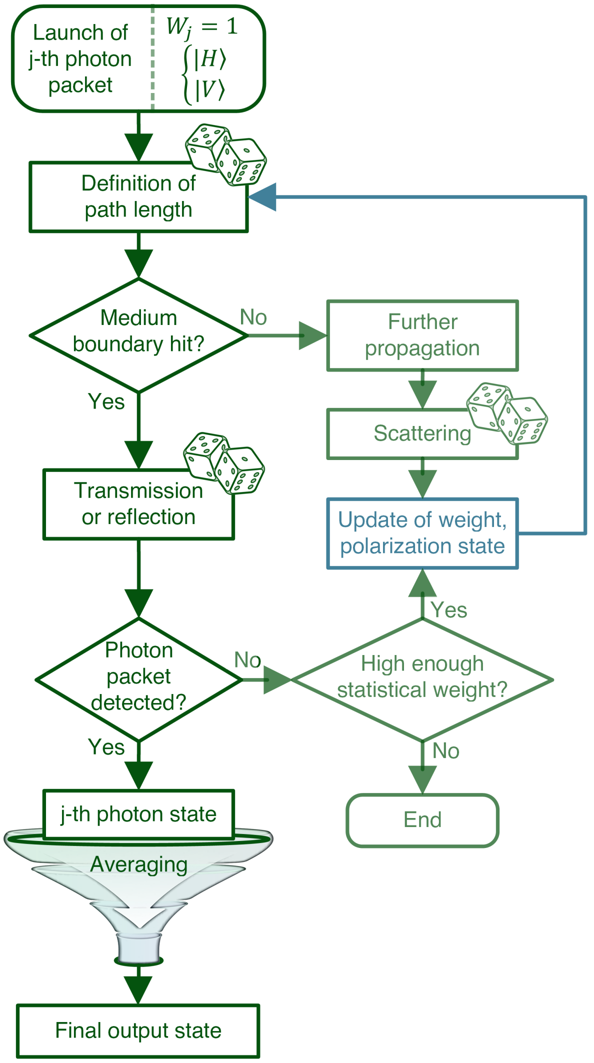


**Fig S1** Conceptual flow chart of the implemented MC model. More details on MC modelling can be found in Ref.[3,4,6]

pixel, also bucket, detector with either infinite or restricted area, acceptance angle and/or exposure time. Hereby, the portion of the photon packets that contribute to the final statistics evaluation can be tuned to correspond to the features of the real experimental setup. This algorithm and its physical background has been extensively covered in our previous works,[3,4,6] and its key parts are depicted in Fig. S1.

### *S1.2 Details on algorithm implementation*

The key steps of the modelling algorithm that we have implemented in the current study is shown in Fig. S1. It is already adapted to model polarization-entangled photon pairs and belongs to one of the main findings of our work.

Firstly, a large amount of photon packets ($N_{inc} > 10^9$) is launched from the light source. We model the uniform distribution of the photon packets within the cross-section of the beam incident on the sample, and so we launch each ($j$-th) of these packets with a unit statistical weight $W_j$. We also supply each photon packet with a polarization vector $\mathbf{P}_0$: for the horizontally polarized state $\mathbf{P}_0 = (1, 0, 0)^T$, and for the vertically polarized state $\mathbf{P}_0 = (0, 1, 0)^T$. Photon packets are launched

from the source and propagate without constraints towards the sample interface: in this work, all photon packets are assumed to be normally incident at the interface, i.e. propagation direction vector $\mathbf{s} = (0, 0, 1)^T$ for all packets. Expressions for the polarization vector above are provided with account for the normal incidence. At the interface, all photon packets undergo transmission with respect to Snell and Fresnel laws.

Secondly, after interface interaction, a probabilistic value of the path length is determined for each photon packet with respect to the Beer-Lambert law:

$$l_i = -\ln\xi/\mu_s.$$

Here, we employ a uniformly distributed random number $\xi \in (0, 1]$ and index of the scattering event $i = [1...N]$, and assume that $\mu_a \ll \mu_s$. The obtained value $l_i$ indicates the distance, for which the photon packet will propagate in the turbid medium until the next scattering event:

$$\mathbf{r}_i = \mathbf{r}_{i-1} + \mathbf{s}_i l_i.$$

At the same time, statistical weight of the photon packet is attenuated as

$$W_i = W_{i-1} e^{-\mu_a l_i}.$$

After the scattering event, the new direction of photon packet propagation $\mathbf{s}_{i+1}$ is randomly chosen with respect to the medium-dependent scattering phase function, which in this case acts as a probability density function. In particular, in this work we use the Henyey-Greenstein (HG) phase function

$$p_{HG}(\cos\theta') = \frac{1}{4\pi}\frac{1-g^2}{(1+g^2-2g\cos\theta')^{3/2}},$$

and its inversion:

$$\cos\theta' = \begin{cases} \frac{1}{2g}\left(1+g^2-\left[\frac{1-g^2}{1-g+2g\xi}\right]^2\right), & \text{if } g > 0,\\ 2\xi - 1, & \text{if } g = 0,\end{cases}$$
$$\varphi' = 2\pi\xi.$$

Here, $\theta'$ and $\varphi'$ are the polar and azimuthal scattering angles in the photon packet reference frame.

We note that if the path of the photon packet crosses the medium boundary (either $z = 0$ or $z = d$, where $d$ is the sample thickness), then instead of the scattering event an interface interaction (i.e. reflection/transmission) event is invoked, which modifies statistical weight with respect to Fresnel law and propagation direction with respect to Snell law. Polarization state of the photon packet can also be updated at this step. However, for various cases it appears possible to postpone the evaluation of the polarization state and perform it only for the photon packets which arrived at the detector, leading e.g. to Eq. (2) in the main body of the paper. We note that this particular equation describes polarization tracing at scattering events and does not account for possible polarization state changes caused by interface reflections.

Finally, photon packets propagate through the turbid medium $0 < z < d$ undergoing a limited amount $N$ of scattering events, and the procedure outlined above repeats $N$ times. Criterion to terminate the propagation of the photon packet originates from the Beer-Lambert law and is either limited by a large amount of scattering events (e.g. $N > 10^3$), or by the negligible statistical

weight (e.g. $W_j < 10^{-4}$) obtained due to attenuation and reflection/transmission events. At each reflection/transmission event, part of the photon packet is always assumed to be reflected and continues propagation in the sample, and the other part is assumed to escape from the sample. For this part of the photon packet, detection conditions are checked. These involve either infinite or restricted area of the detector, acceptance angle and other possible limitations.[3] Those $N_{ph}$ photon packets that arrive at the detector and satisfy the detection conditions finally contribute to the statistics.

Our polarization tracing procedure (2) defined in the main body of the paper requires for both statistical weight and power of the Rayleigh factor $\Gamma_R = 2/\left(1+\overline{\cos^2\theta}\right)$ of the photon packet to be accounted for along with the detected polarization state $\mathbf{P}_N$ in order to correctly determine its polarization-projected intensity value.[4,6–8] Here, $\overline{\cos^2\theta}$ is the square cosine of the scattering angle weighted by the single scattering cross-section.[6] For instance, in the case of the photon detected with $\mathbf{X}_j = \mathfrak{m}_j \boldsymbol{\varepsilon}_H + \mathfrak{n}_j \boldsymbol{\varepsilon}_V$ state $H$ and $V$ intensity projections can be evaluated as:[3,6]

$$I_H\left(\mathbf{X}_j\right) = W_j \mathfrak{m}_j^2 \Gamma_R^{N_j}, \quad I_V\left(\mathbf{X}_j\right) = W_j \mathfrak{n}_j^2 \Gamma_R^{N_j}. \tag{S.1}$$

Here, $W_j$ is the detected statistical weight of the $j$-th photon packet which has propagated through the turbid sample, $N_j$ corresponds to the amount of scattering events along the $j$-the photon packet trajectory prior to the detection event, and $\Gamma_R$ is derived from the optical theorem in Born approximation.[4,7,8] We note that in these particular expressions, elements of $\mathbf{X}_j$ are assumed to be real-valued, but in general Jones formalism they can be complex-valued. In this case, square values $\mathfrak{m}^2, \mathfrak{n}^2$ will be replaced by $\mathfrak{m} \cdot \mathfrak{m}^*, \mathfrak{n} \cdot \mathfrak{n}^*$ products. With the above mentioned in mind, expressions which have the form of (S.1) can be rewritten in the Dirac bra-ket terms following the Eq. (21) in the main body of the paper. Correspondingly, averaging procedure for these $N_{ph} < N_{inc}$ single photon packets can be written in exactly the same way as Eq. (22) in the main body of the paper by replacing two-photon state $\Phi$ with the single photon state $\phi$.

In our MC modelling, we employ the framework of iterative solution to Bethe-Salpeter equation (BSE framework) and thus can track both horizontal $\boldsymbol{\varepsilon}_H$ and vertical $\boldsymbol{\varepsilon}_V$ states along any photon packet trajectory simultaneously and independently, while assuming Rayleigh-Gans-Debye approximation. In fact, this means tracking both polarization states along the same trajectory, which, generally speaking, might change at one of the later scattering events if the medium exhibits polarization selectivity.

### *S1.3 Relation of polarization vector to Jones vector*

In this section, we provide details on the relation between Jones vector and polarization vector simulated by the BSE-based MC. For this purpose, in addition to the so-called laboratory Cartesian coordinates $(x, y, z)$ associated with the sample, we introduce local Cartesian coordinates $(x', y', z')$, where $z'$ axis is always collinear with the photon packet propagation direction $\mathbf{s} = (s_x, s_y, s_z)$. The $(x', y')$ plane in these prime coordinates defines the reference plane of the photon packet.

Jones vector by definition is always expressed in the reference plane $\boldsymbol{\varepsilon} = (E_{x'}, E_{y'})^T$ and corresponds to the prime electric vector $\mathbf{E}' = (E_{x'}, E_{y'}, 0)^T$. When expressed in terms of the laboratory Cartesian coordinates, the same electric vector can generally obtain third component

$\mathbf{E} = (E_x, E_y, E_z)^T$. This can be demonstrated by utilizing the proper transition matrix:

$$\mathbf{P} \propto \mathbf{E} = \begin{pmatrix} E_x \\ E_y \\ E_z \end{pmatrix} = \begin{pmatrix} \cos\theta\cos\varphi & -\sin\varphi & \sin\theta\cos\varphi \\ \cos\theta\sin\varphi & \cos\varphi & \sin\theta\sin\varphi \\ -\sin\theta & 0 & \cos\theta \end{pmatrix} \begin{pmatrix} E_{x'} \\ E_{y'} \\ 0 \end{pmatrix}.$$

Here, $\theta = \arccos(s_z/|\mathrm{s}|)$ is a polar angle of the photon packet direction vector s and $\varphi$ is an azimuthal angle of this vector expressed in terms of the spherical coordinate system which corresponds to the introduced laboratory Cartesian coordinates. To track evolution of the polarization state of the photons experiencing scattering, we have introduced vector $\mathbf{P}$. We do so in the laboratory Cartesian coordinates, and with the proportionality sign we emphasize that $\mathbf{P}$ vector corresponds to the $\mathbf{E}$ direction.[4,6–8] As indicated both in the previous section and in the main body of the paper, it is necessary to account for the statistical weight of the photon packet and for the power of the Rayleigh factor $\Gamma_R$ in order to evaluate corresponding intensity projections.

Thereby, in this work we rely on the fact that it is always possible to interchange between $(x, y, z)$ and $(x', y', z')$ coordinate frames by using proper transition matrix. We point out that the connection between the introduced $\mathbf{E}'$ and its counterpart $\mathbf{E}$ is always known. This connection also enables to link Jones vector $\boldsymbol{\varepsilon}$ and electric field $\mathbf{E}$ vectors, and, correspondingly, $\boldsymbol{\varepsilon}$ and $\mathbf{P}$ vectors for each photon packet. Given that $\mathbf{P}$ is always orthogonal to the propagation direction of the photon packet, Jones vector components can always be reconstructed by using the reverse transition matrix.[9]

## S2 Experimental implementation

### *S2.1 Samples*

As samples of turbid medium for current study we selected tissue mimicking phantoms. The latter appear each as a turbid polymer film with scattering centers (nanoparticles) homogeneously allocated within the volume of the phantom.[10] The material used for the particles, their size and distribution profile are responsible for achieving different scattering properties of the synthesized medium. Herein, the resultant density of the scattering centers and scattering anisotropy of the manufactured samples can closely mimic optical properties of the real biomatter, like skin or inner tissue. At the same time, low levels of scattering centers density in such samples match well to poor atmospheric conditions, e.g. particulate polluted atmosphere in urban areas.

For the reported studies, we manufactured a series of thin ($d = 300$ $\mu$m thick) tissue phantoms exhibiting varying scattering coefficient $\mu_s$: from relatively low as for polluted air[11] to high value as for human tissue.[12] Other optical properties of the samples were kept similar: refractive index $n$ = 1.47, low absorption coefficient $\mu_a$ on the order of 0.1 mm$^{-1}$, and forward scattering anisotropy factor $g$ = 0.65. Besides scattering coefficient $\mu_s$, we also use reduced scattering coefficient $\mu_s'$, and transport mean free path $l^*$, which considering the low level of absorption can be defined as $l^* = 1/\mu_s' = \mu_s^{-1}(1-g)^{-1}$.[1] The scattering properties of the phantoms have been selected so that the effective thickness $d/l^*$ of the samples gradually reaches $1.0$: $\mu_s' =$ 0.45, 0.96, 1.55, 2.44, and 3.34 mm$^{-1}$. As a reference sample we use a polymer matrix without ZnO nanoparticles and thus characterized by negligible scattering coefficient. For handling, each sample is mounted between two standard glass microslides.

*S2.2 Realized optical arrangement and measurement procedure*

For experimental studies of scattering of the entangled photons we perform a sequential reconstruction of the quantum state which either was perturbed by the sample or not. The instrument used for this purpose consists of the source of polarization-entangled photon pairs and the optical setup for quantum state characterization. The conceptual design of the corresponding optical arrangement is shown in Fig. 2 in the main body of the paper.

First, the generation of the probing quantum state is performed, where we target at the Bell state in the form $|\Psi^+\rangle = 1/\sqrt{2}(|HV\rangle + |VH\rangle)$. We employ two identical periodically-poled KTP (Potassium Titanyl Phosphate) crystals, each serving for generation of a pair of orthogonally polarized photons within a type-II event of spontaneous parametric down-conversion (SPDC). These crystals are introduced with their optical axes oriented orthogonally into a polarization Mach-Zehnder interferometer and the optical paths of the generated photon pairs are matched to achieve indistinguishability.[13] The wavelength-degenerate pairs are created at 810 nm, exit the interferometer and the resultant biphoton state is characterized using the well-known approach of quantum state tomography (QST) including maximum likelihood estimation method.[14,15] The fidelity of the realized state with respect to the nominal Bell state is obtained at the level of 0.97 by proper control of the spatial and temporal walk-off between the beams.[16,17] The described part of the setup is omitted in Fig. 2.

The second part of the instrument is used for both initial source characterization and experiments with tissue phantoms. For this, photon pairs are split into two spatially remote optical channels with each containing a polarization projector (also polarization state analyzer) and a fiber-coupled single photon counting module (detector). The latter is supplemented with a single-mode fiber with numerical aperture of 0.13. The polarization projector in each channel is realized with a quarter-wave plate (QWP) and a linear polarizer (LP), and is responsible for projecting the state to be analyzed to one of the basis states: $|H\rangle$ for horizontal, $|V\rangle$ for vertical, $|D\rangle$ for +45°, $|A\rangle$ -45°, $|R\rangle$ for right-circular, and $|L\rangle$ for left circular polarizations. For each of these projective measurements, both QWP (with its fast axis) and LP (with its transmission axis) are oriented at different angles with respect to the global vertical direction. For complete tomographic reconstruction of the quantum state – either as generated by the source or modified by the sample in the optical path – 16 combinations of polarization projections following Ref.[14] are implemented.

The detectors of single photons in both channels are connected to a time tagging device for counting the coincidence events. These correspond to the photon pairs reaching the detectors within a narrow time window, also coincidence window, which relates these photons to the same event of generation. Providing the comparable level of coincidences counted for different independent polarization bases, one can claim them entangled. In the experiments, the coincidence events between the channels are accumulated for 10 s within the coincidence window of 3 ns for each combination of polarization projections in a sequential manner. After correction for accidental counts, intensity drift, and detector efficiency,[15] the QST algorithm for one detector per channel is employed including the maximum likelihood estimation method.[15]

The samples under study were introduced into one of the optical channels (signal, or sample, channel) without extra condenser or objective lens. Hereby, the sample is illuminated with a collimated beam of approx. 1 mm in diameter. This allows to probe a relatively large area of the homogeneous phantom and thus obtain an integral response from the sample (phantom laterial dimensions are approx. 20 mm $\times$ 70 mm) and extra minimize the influence of any contamination of

the sample or localized artifacts.

Accounting for relatively strong scattering occurring in the tissue phantoms, an auxiliary low-focusing lens is introduced between the sample and polarization projector in the signal channel to enhance the coupling of the photons with changed trajectory of propagation to the single-mode-fiber input of the detector. The other, reference, channel of the instrument remains unchanged as for the case of photon pair source characterization.

To study the behaviour of the entangled photons when passing through a turbid medium and to compare later the experimental and simulation results, we have reconstructed the experimentally measured density matrices of the probing state, output state after the photons in the signal channel are passing through the auxiliary lens only, and the state carrying the information of both the lens and the sample.

### *S2.3 Measurement of the phase retardation effects on the density matrix*

Density matrix of the pure Bell state $|\Psi^{+}\rangle$ is well-known to be a real $4 \times 4$ matrix with zero side elements and four central elements equal to 0.5. This corresponds to the case of maximally entangled state characterized by unit concurrence and zero linear entropy. One of the special cases important for our research is the impact of a phase retarder on this density matrix. Namely, if we put a QWP inside the signal channel sketched in Fig. 2, we will expectedly observe a density matrix with the same characteristics and absolute values of the matrix elements, but with nonzero imaginary parts of the anti-diagonal elements:

$$\hat{\rho}^{(QWP)} = \begin{pmatrix} 0 & 0 & 0 & 0 \\ 0 & 0.5 & -0.5j & 0 \\ 0 & 0.5j & 0.5 & 0 \\ 0 & 0 & 0 & 0 \end{pmatrix}.$$

This corresponds to the scenario when $\boldsymbol{\varepsilon}_H$-polarized photons pass through the waveplate without change, while $\boldsymbol{\varepsilon}_V$-polarized photons acquire phase shift $\delta = \lambda/4$ due to birefringence. In terms of Jones calculus in our model, this is expressed as

$$\mathbf{X} = \boldsymbol{\varepsilon}_H = \left( \begin{array}{c} 1 \\ 0 \end{array} \right), \quad \mathbf{Y} = \boldsymbol{\varepsilon}_V \exp\left(jk\delta\right) = \left( \begin{array}{c} 0 \\ j \end{array} \right),$$

and $\hat{\rho}^{(QWP)}$ can be immediately obtained from these expressions via Eq. (17) in the main body of the paper. As expected, no change is observed in the diagonal elements of the matrix which correspond to the probabilities of the $|HV\rangle$ and $|VH\rangle$ states while the correlations between them (off-axis elements) are transferred from the real to the imaginary part. The latter indicates the phase delay introduced by the QWP.

Understanding of this effect is important when interpreting the density matrices measured for samples under study. As already mentioned in Sec. S2.2, in the experiments with scattering samples an auxiliary low-focusing lens was found necessary to compensate for the decreased collection of the scattered photons. We have, though, noticed that if a lens is introduced into the optical path, the detected state changes and the density matrix of the considered Bell state acquires imaginary anti-diagonal elements, as if birefringence was present in the system (see Figure S2a). Also, the absolute values of the diagonal elements cease to be equal (difference on the level of 1.5%). This

phenomenon could be explained by the fact that the lens influences both the polarization state and path lengths of the incident light,[18] as well as by the induced birefringence which could appear while mounting the lens.

In order to account for the lens influence on the density matrix in the simulation model, we made a fit of the simulation parameters which leads to the computed density matrix that is similar to the measured one in presence of the lens (see Figure S2b). In fact, such a fit endows the lens with properties of polarization selective transmission and birefringence. The values of the defined fitting parameters indicate that the presence of the lens in the optical path could result in slightly preferred transmission of the horizontal polarization and exhibit extremely low ($\lambda/26$) level of birefringence (or phase delay influenced by other effects). The latter is not commonly considered for most of the applications using classical states of light taking into account the negligibility of the effect. It appears, though, critical when dealing with polarization-entangled photon pairs and indicates potentially enhanced sensitivity of the measurement using such and further non-classical states of light.[19] The discussed issue will be further investigated in our future studies while for the current work we employ the fitted model of the lens.

Due to the indicated lens influence, as well as due to other possible effects, characteristics of the measured density matrix differ from the ones that correspond to the pure Bell state. However, nonzero phase retardation itself does not impact the purity of the state.[20] This leads us to the conclusion that in simulations we have to consider an initially mixed state which can be defined by Eq. (11) in the main body of the paper:

$$\hat{\rho} = \frac{19}{20}|\Psi^{+}\rangle\langle\Psi^{+}| + \frac{1}{20}|\Psi^{-}\rangle\langle\Psi^{-}|. \tag{S.2}$$

Probability values $[19/20, 1/20]$ in the expression (S.2) are fit to best match the characteristics of the density matrix measured without the sample: the obtained $\hat{\rho}$ exhibits concurrence, linear

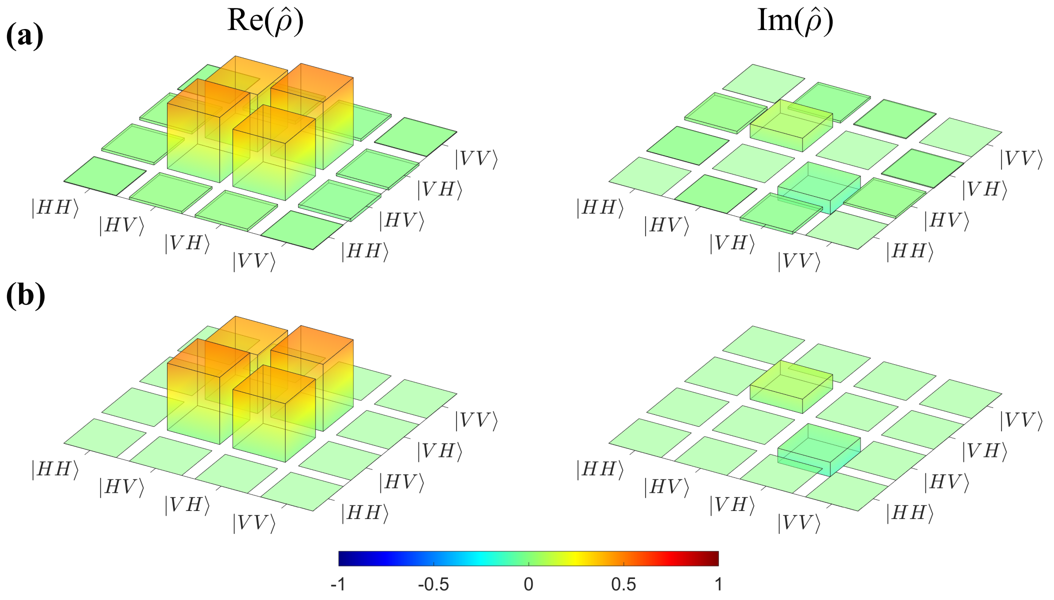


**Fig S2** (a) Measured and (b) simulated density matrix of the state without scattering sample. Simulated matrix accounts for the phase delay $\delta = -\lambda/26$ which might be explained among others by the possible induced birefringence in the auxiliary lens, as well as for the mix of two linearly independent Bell states defined by Eq. (S.2).

entropy and dephasing values similar to the ones observed in the experimental measurements. With account for the indicated phase delay, we subsequently simulate $|\Psi^+\rangle$ and $|\Psi^-\rangle$ within our MC approach, reconstruct corresponding ensemble density matrices $\hat{\rho}^+$, $\hat{\rho}^-$ via Eq. (23) in the main body of the paper, and evaluate density matrix of the mixed state with various probability coefficients.

*References*


1 V. V. Tuchin, *Tissue Optics: Light Scattering Methods and Instruments for Medical Diagnostics*, SPIE Press, Bellingham, Washington, 3rd ed. (2015).

2 M. I. Mishchenko, "Vector radiative transfer equation for arbitrarily shaped and arbitrarily oriented particles: a microphysical derivation from statistical electromagnetics," *Appl. Opt.* **41**, 7114–7134 (2002).

3 I. Lopushenko, O. Sieryi, A. Bykov, *et al.*, "Exploring the evolution of circular polarized light backscattered from turbid tissue-like disperse medium utilizing generalized Monte Carlo modeling approach with a combined use of Jones and Stokes-Mueller formalisms," *J. Biomed. Opt.* **29**(5) (2024).

4 I. Meglinski and A. Doronin, "Monte Carlo Modeling of Photon Migration for the Needs of Biomedical Optics and Biophotonics," in *Advanced Biophotonics: Tissue Optical Sectioning*, R. K. Wang and V. V. Tuchin, Eds., ch. 1, 1–72, CRC Press, Boca Raton (2013).

5 I. Meglinski, I. Lopushenko, A. Sdobnov, *et al.*, "Phase preservation of orbital angular momentum of light in multiple scattering environment," *Light Sci. Appl.* **13**, 214 (2024).

6 V. Kuz'min and I. Meglinski, "Numerical simulation of coherent backscattering and temporal intensity correlations in random media," *Quantum Electron.* **36**(11), 990 (2006).

7 E. Akkermans, P. E. Wolf, R. Maynard, *et al.*, "Theoretical study of the coherent backscattering of light by disordered media," *J. Phys. France* **49**, 77–98 (1988).

8 I. Meglinski, V. L. Kuzmin, D. Y. Churmakov, *et al.*, "Monte Carlo simulation of coherent effects in multiple scattering," *Proc. R. Soc. A* **461**, 43 – 53 (2005).

9 L. Mandel and E. Wolf, *Optical coherence and quantum optics*, Cambridge University Press, Cambridge (1995).

10 O. Sieryi, A. Popov, V. Kalchenko, *et al.*, "Tissue-mimicking phantoms for biomedical applications," *Proc. SPIE* **11363**, 1136312 (2020).

11 A. Marshak and A. B. Davis, Eds., *3D Radiative Transfer in Cloudy Atmospheres*, Springer, Berlin (2005).

12 A. N. Bashkatov, E. A. Genina, and V. V. Tuchin, "Optical properties of skin, subcutaneous, and muscle tissues: A review," *J. Innov. Opt. Health Sci.* **04**(01), 9–38 (2011).

13 R. Horn and T. Jennewein, "Auto-balancing and robust interferometer designs for polarization entangled photon sources," *Opt. Express* **27**(12), 17369–17376 (2019).

14 D. F. V. James, P. G. Kwiat, W. J. Munro, *et al.*, "Measurement of qubits," *Phys. Rev. A* **64**, 052312 (2001).

15 M. Paris and J. Řeháček, Eds., *Quantum State Estimation*, Springer Berlin Heidelberg, Berlin, Heidelberg (2004).

16 S. Oh and T. Jennewein, "Polarization entanglement with highly non-degenerate photon pairs enhanced by effective walk-off compensation method," (2024).

17 V. R. Besaga, L. Zhang, A. Vega, *et al.*, “Nonlocal quantum differentiation between polarization objects using entanglement,” *APL Photon.* **9**, 041301 (2024).

18 Y. Shen, B. Chen, C. He, *et al.*, “Polarization aberrations in high-numerical-aperture lens systems and their effects on vectorial-information sensing,” *Remote Sensing* **14**(8) (2022).

19 A. Pedram, V. R. Besaga, F. Setzpfandt, *et al.*, “Nonlocality enhanced precision in quantum polarimetry via entangled photons,” *Adv. Quantum Technol.* , 2400059 (2024).

20 A. G. White, D. F. V. James, P. H. Eberhard, *et al.*, “Nonmaximally Entangled States: Production, Characterization, and Utilization,” *Phys. Rev. Lett.* **83**(16), 3103–3107 (1999).
